# Supplementary material for: Language Embeddings for Typology and Cross-lingual Transfer Learning
Source: arXiv:2106.02082 source file (2021-06-03)
Supplement: Supplementary file 1 [file appendix_XNLI.tex]

\clearpage
\subsection{XNLI} \label{app_xnli}
\begin{table}[!h]
\small
\centering
\resizebox{\textwidth}{!}{
\begin{tabular}{l|ccccccccc|c}
\toprule
& fr             & es    & de    & el    & bg    & ru    & tr    & ar    & vi  & avg.  \\ 
\midrule

Wiki baseline & 59.42 & 60.70 &	59.66 &	52.73 &	58.80 &	57.17 &	51.42 &	51.28 &	42.75 &	54.88 \\
\midrule
\multicolumn{11}{l}{\textit{Original language embeddings}} \\
\midrule
XLM parallel lang\_emb & 60.84 & 62.22 & 60.88 & 51.76 & 57.54 & 56.97 & 50.82 & 53.61 & \textbf{47.03} & 55.74 \\
XLM mono lang\_emb & 60.96 & 61.38 & 60.06 & 52.28 & 58.82 & 57.84 & 50.72 & 54.53 & 46.39 & 55.89 \\
Wiki lang\_emb & 60.40 & 63.23 & 60.62 & \textbf{53.67} & 58.90 & 58.00 & 50.96 & \textbf{54.65} & 45.37 & \textbf{56.20} \\
\midrule
\multicolumn{11}{l}{\textit{Converted language embeddings to 50 dimensions with a learned linear transformation }} \\
\midrule
Conv. XLM parallel & \textbf{61.08} & 63.19 & 60.54 & 53.01 & 57.66 & 57.54 & 50.46 & 54.09 & 44.69 & 55.81 \\
Conv. XLM mono & 60.32 & 61.28 & 60.32 & 51.56 & \textbf{59.26} & \textbf{58.2} & 49.94 & 53.39 & 44.59 & 55.43 \\
Conv. Wiki & 60.96 & \textbf{63.51} & \textbf{60.94} & 53.53 & 58.48 & 57.33 & \textbf{51.78} & 53.25 & 45.67 & 56.16 \\

\bottomrule
\end{tabular}
}
% \end{center}
\caption{\label{app_xnli_results}  Comparison with different language embeddings on the XNLI task. All the embeddings are generated using Wikipedia data. Wiki baseline does not use language embedding. XLM parallel lang\_emb is extracted from \citet{xlm} pre-trained on 15 languages using parallel data. XLM mono lang\_emb is pre-trained on the same 29 languages with the same Wiki data as our experiment. Language embeddings from XLM has a dimension to 1024. In order to study the influence of dimension, we train a linear layer to convert the learned language embedding to 50 dimensions. All experiments with language embeddings show better performance over the baseline, which does not use language embeddings.}
\end{table}
